# Supplementary material for: Ergodicity breaking in rapidly rotating C60 fullerenes
Source: arXiv:2305.05324 source file (2023-05-09)

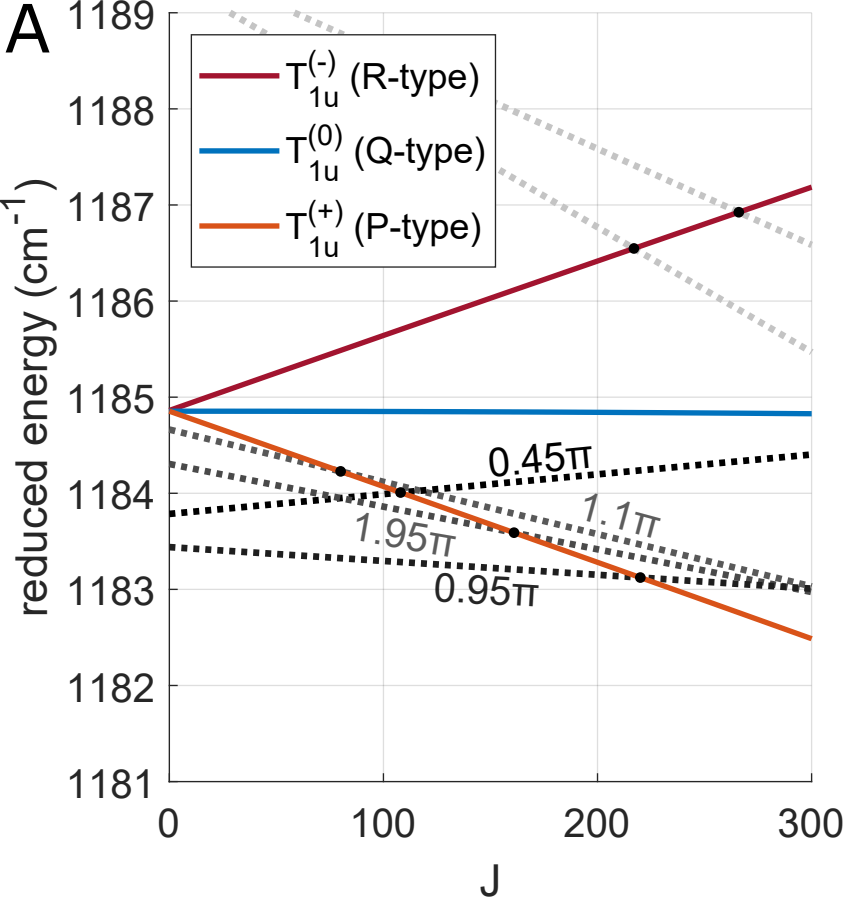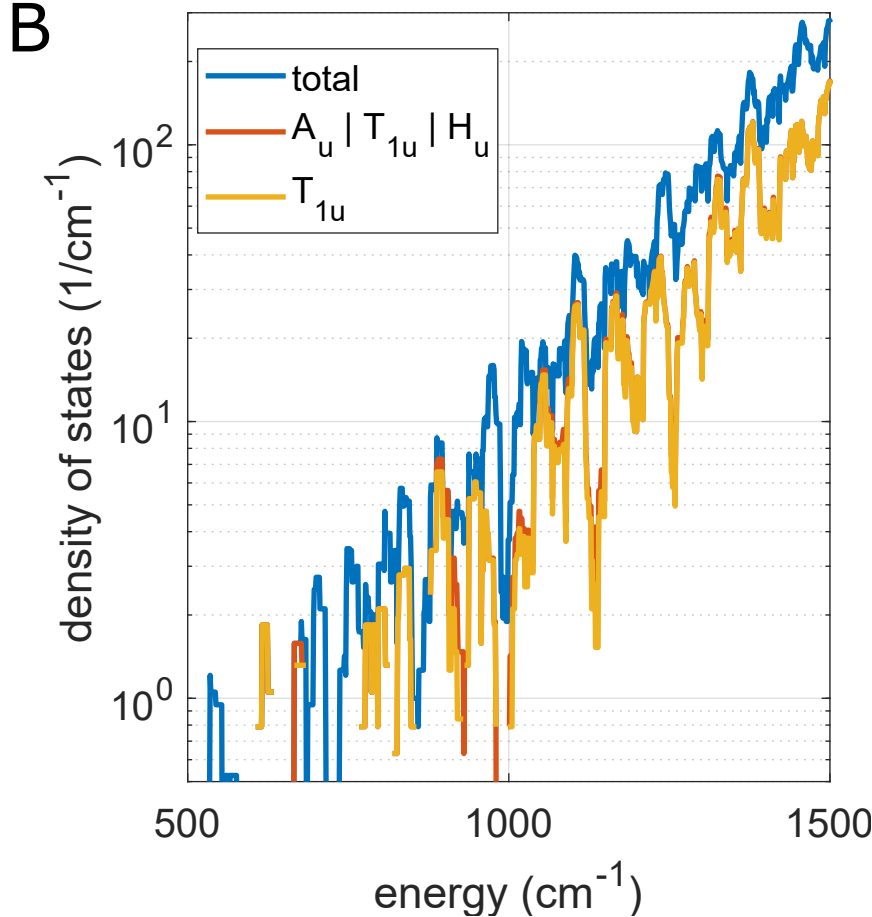

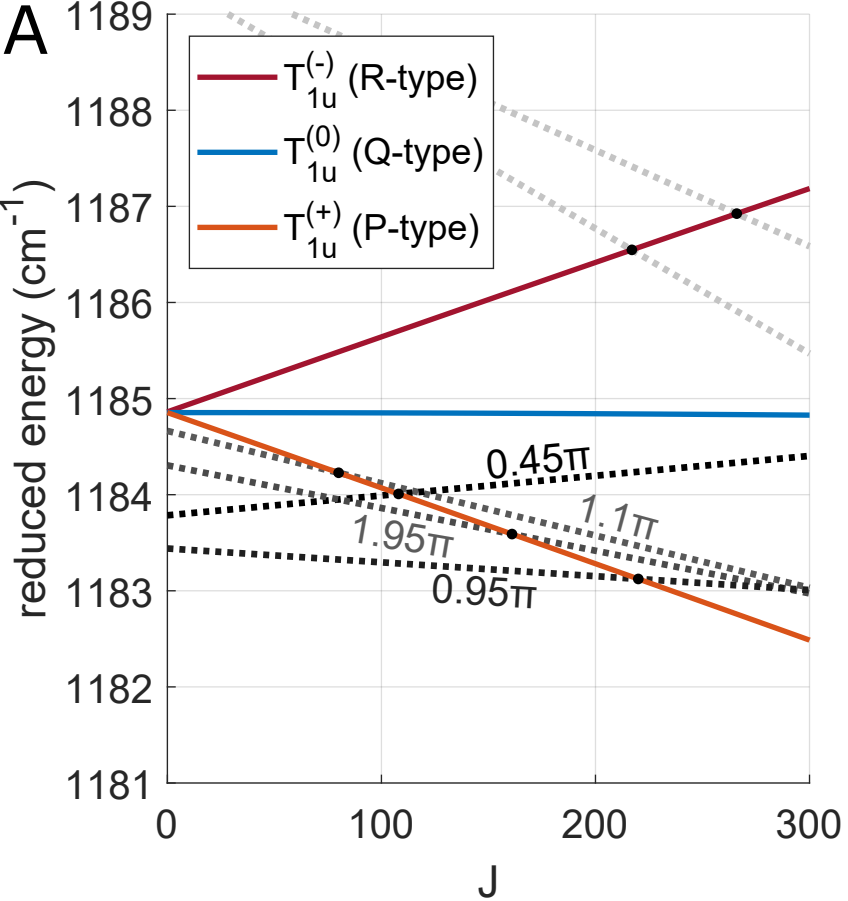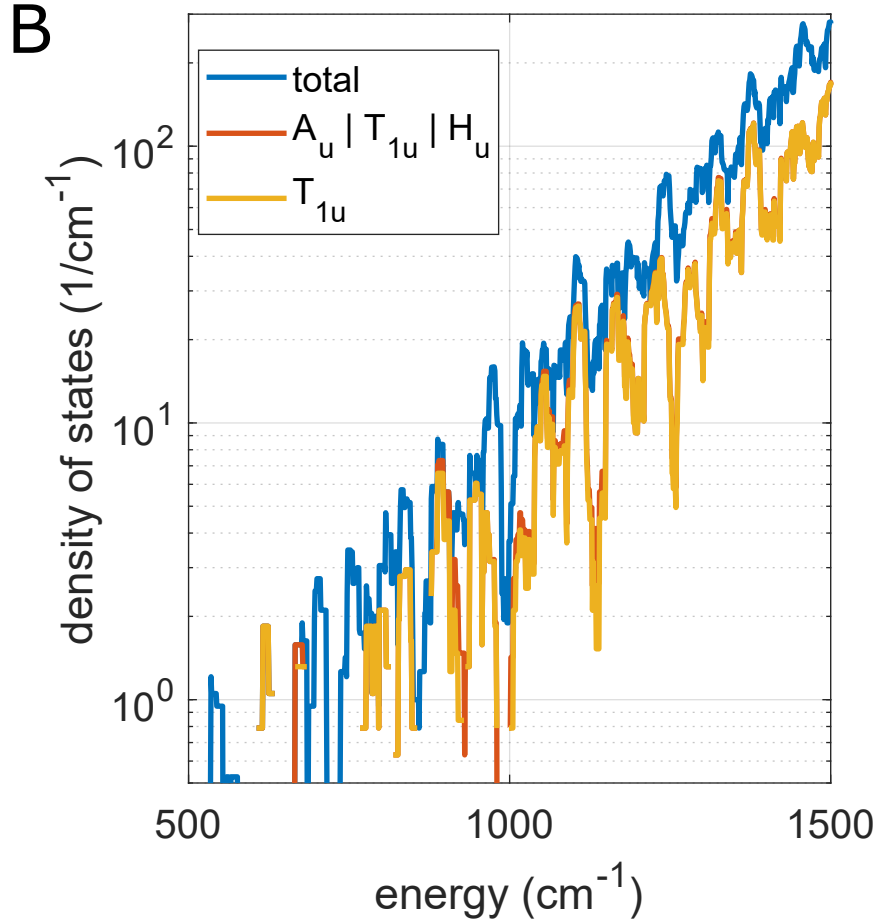

Supplement: Supplementary file 1 [file SI_dark_states.pdf]
