# Supplementary material for: Ergodicity breaking in rapidly rotating C60 fullerenes
Source: arXiv:2305.05324 source file (2023-05-09)

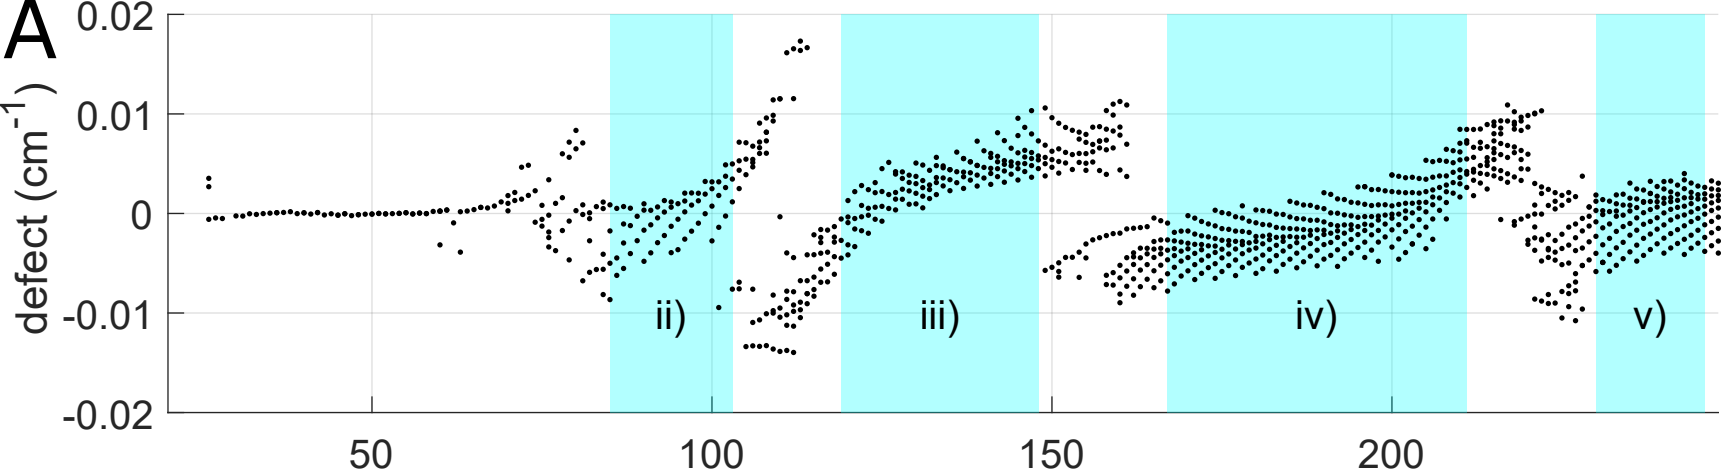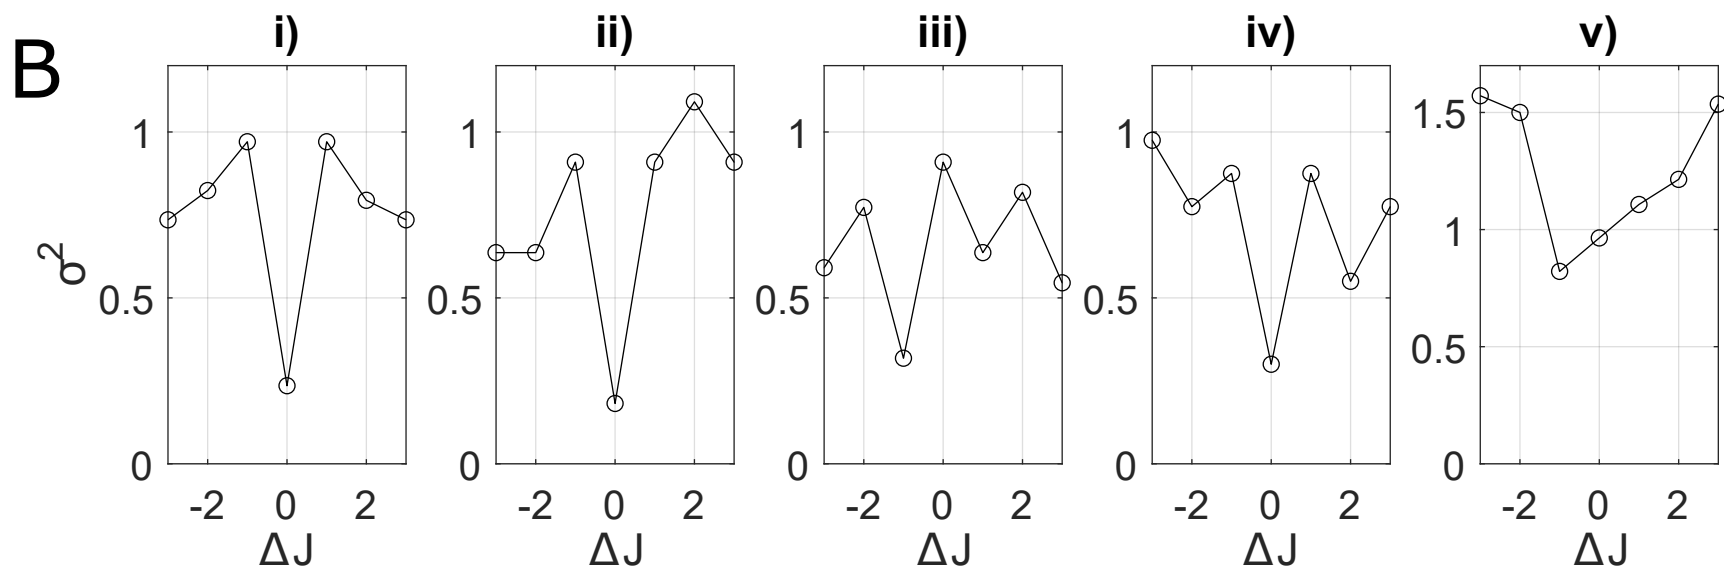



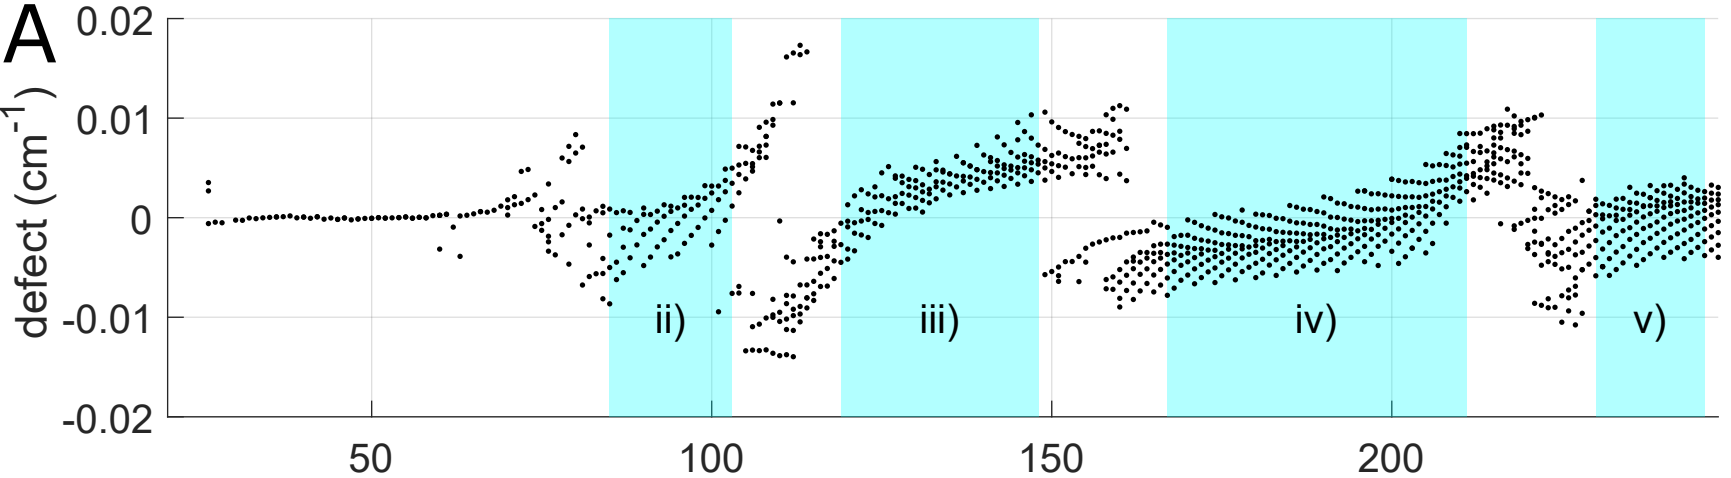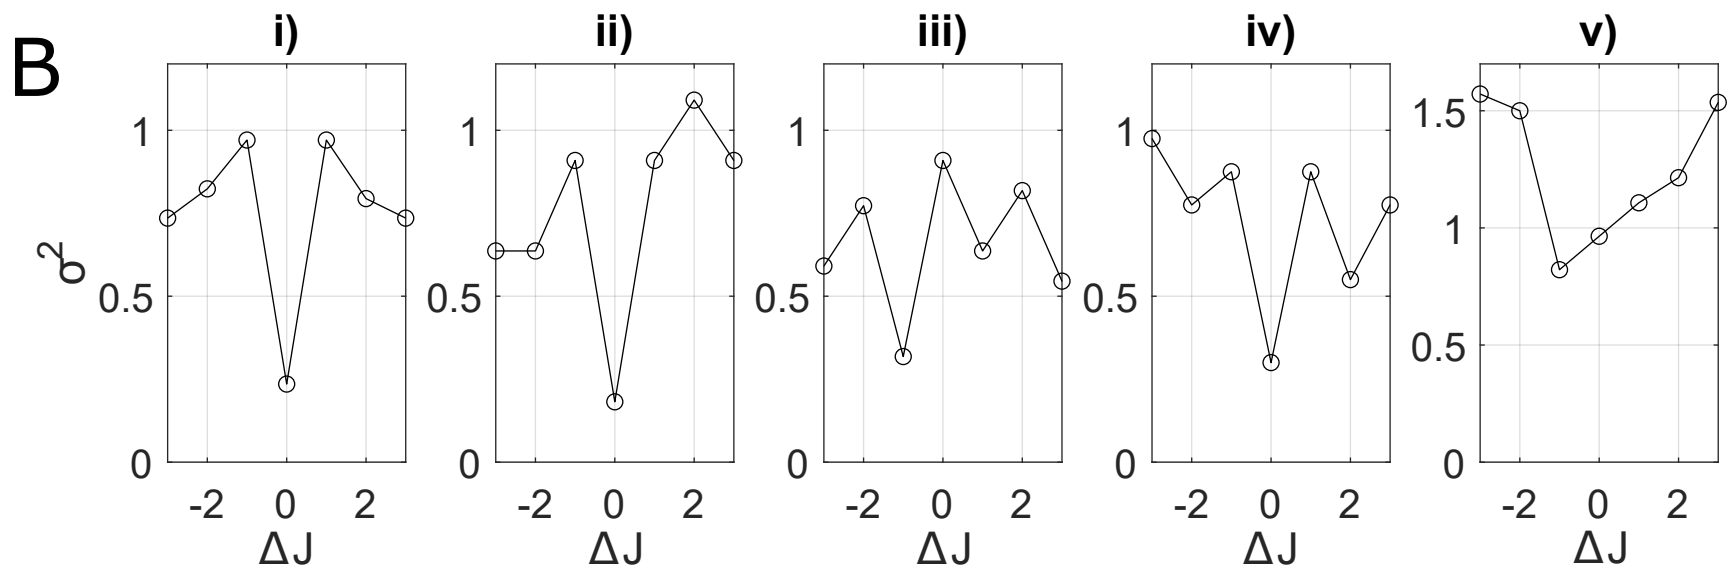

Supplement: Supplementary file 2 [file SI_defect_plot.pdf]
