# Supplementary material for: Ergodicity breaking in rapidly rotating C60 fullerenes
Source: arXiv:2305.05324 source file (2023-05-09)

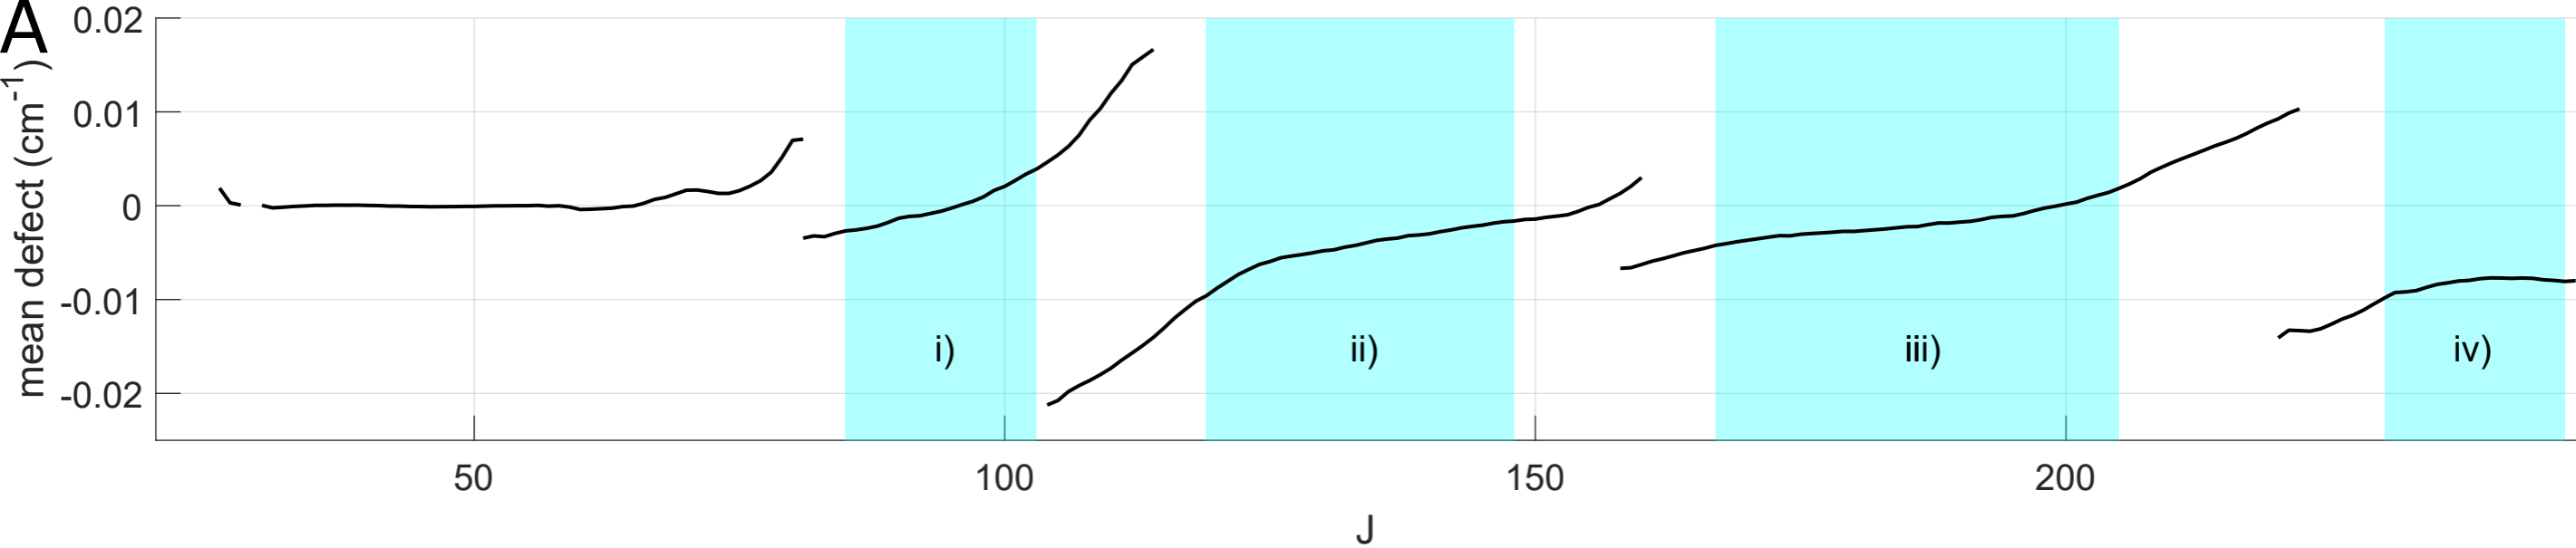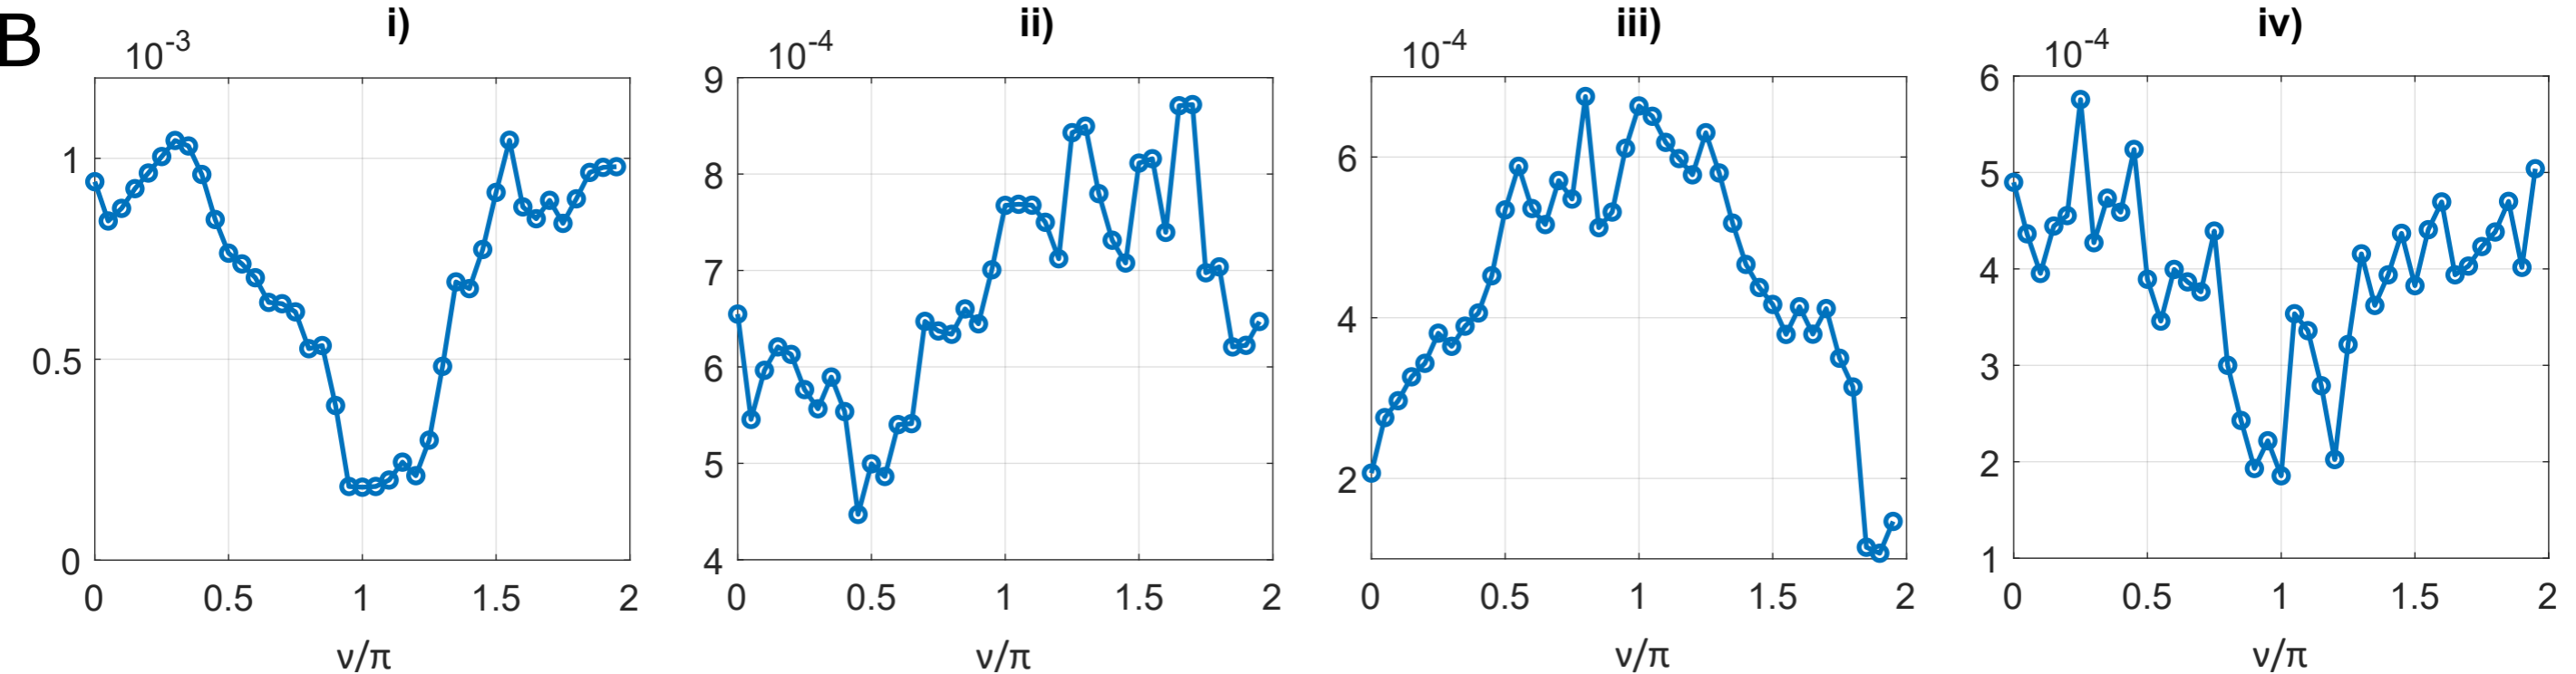

Supplement: Supplementary file 3 [file SI_optimize_nu_pcreg.pdf]
